# Supplementary material for: EdgeSight: Enabling Modeless and Cost-Efficient Inference at the Edge
Source: arXiv:2405.19213 source file (2025-01-15)
Supplement: Supplementary file 1 [file appendix.tex]

\section{Appendix}

Appendix
